# Supplementary material for: Leveraging Generative AI for Urban Digital Twins: A Scoping Review on the Autonomous Generation of Urban Data, Scenarios, Designs, and 3D City Models for Smart City Advancement
Source: arXiv:2405.19464 source file (2024-08-06)
Supplement: Supplementary file 1 [file 70-appendix.tex]

\section{Appendix} \label{sec:Appendix}
